# Supplementary material for: Polybot: Training One Policy Across Robots While Embracing Variability
Source: arXiv:2307.03719 source file (2023-07-07)
Supplement: Supplementary file 1 [file 8-appendix.tex]

% this needs to be separated from the main paper for submission
\newpage
\appendix
\section{Appendix}
\subsection{Implementation Details and Hyperparameters}

We now provide details of the various hyperparameters used in our experiments. 
\begin{itemize}
    \item \textbf{AWAC}: Our hyperparameters for AWAC are listed in Table~\ref{tab:awac_sim_hparams}.
    \item \textbf{Multi-Task RL}: We use the same hyperparameters as AWAC. We modify the policy and Q function architectures to accept two additional one-hot task indices. These task indices go unused during offline learning, but we use them to label the new data during online training. 
    \item \textbf{R3L}: For this method, we keep the same RL hyperparameters as Table~\ref{tab:awac_sim_hparams}. For the RND networks we use the same CNN architecture as the policy and Q function networks but set the output dimension to 5.
    \item \textbf{Oracle}: For this method, we keep the same RL hyperparameters as Table~\ref{tab:awac_sim_hparams}, but learn a single-task policy. The offline dataset consists of 512 trajectories.
    \item \textbf{ARIEL}: During online fine-tuning on new tasks with \methodName, we keep the same hyperparameters as Table~\ref{tab:awac_sim_hparams}, but use the path lengths listed in Table \ref{tab:env_hparams1}, \ref{tab:env_hparams2}, and \ref{tab:env_hparams3}. For CEM, we use a Gaussian mixture model as the sampling distributions with a number of components equal to the number of tasks in the prior data. In simulation, we update the sampling distributions every 10 trajectories, fitting them to the $J = 25$ most recent successful task embeddings. In the real world domains, we update the sampling distributions every 10 trajectories, fitting them to the $J = 10$ most recent successful task embeddings.
\end{itemize}

\begin{table}[!htbp]
    \begin{center}
    \begin{tabular}{lr}
    \hline
     Hyperparameter & Value\\
    \hline
     Target Network Update Frequency & 1 step \\
     Discount Factor $\gamma$ & 0.9666 \\
     Beta & 0.01 \\
     Batch Size & 64 \\
     Meta Batch Size & 8 \\
     Soft Target $\tau$ & $5e^{-3}$\\
     Policy Learning Rate & $3e^{-4}$ \\
     Q Function Learning Rate & $3e^{-4}$ \\
     Reward Scale & 1.0 \\
     Alpha & 0.0 \\
     Policy Weight Decay & $1e^{-4}$\\
     Clip Score & 0.5 \\
    \hline
    \end{tabular}
    \end{center}
    \caption{Hyperparameters for AWAC for Simulated Domains}
    \label{tab:awac_sim_hparams}
\end{table}

\subsection{Simulation}
We utilize a Pybullet-based simulation \cite{coumans2016pybullet} containing 3D object models from the Shapenet dataset \cite{shapenet} to test our method on diverse objects. We utilize a near-convex decomposition of the models in order to maintain good contact physics. The following is an example trajectory picking up an cylindrical object and placing it into a container. 
\begin{figure}[!htbp]
    \centering
    \vspace{0.1cm}
    \includegraphics[width=0.4\textwidth]{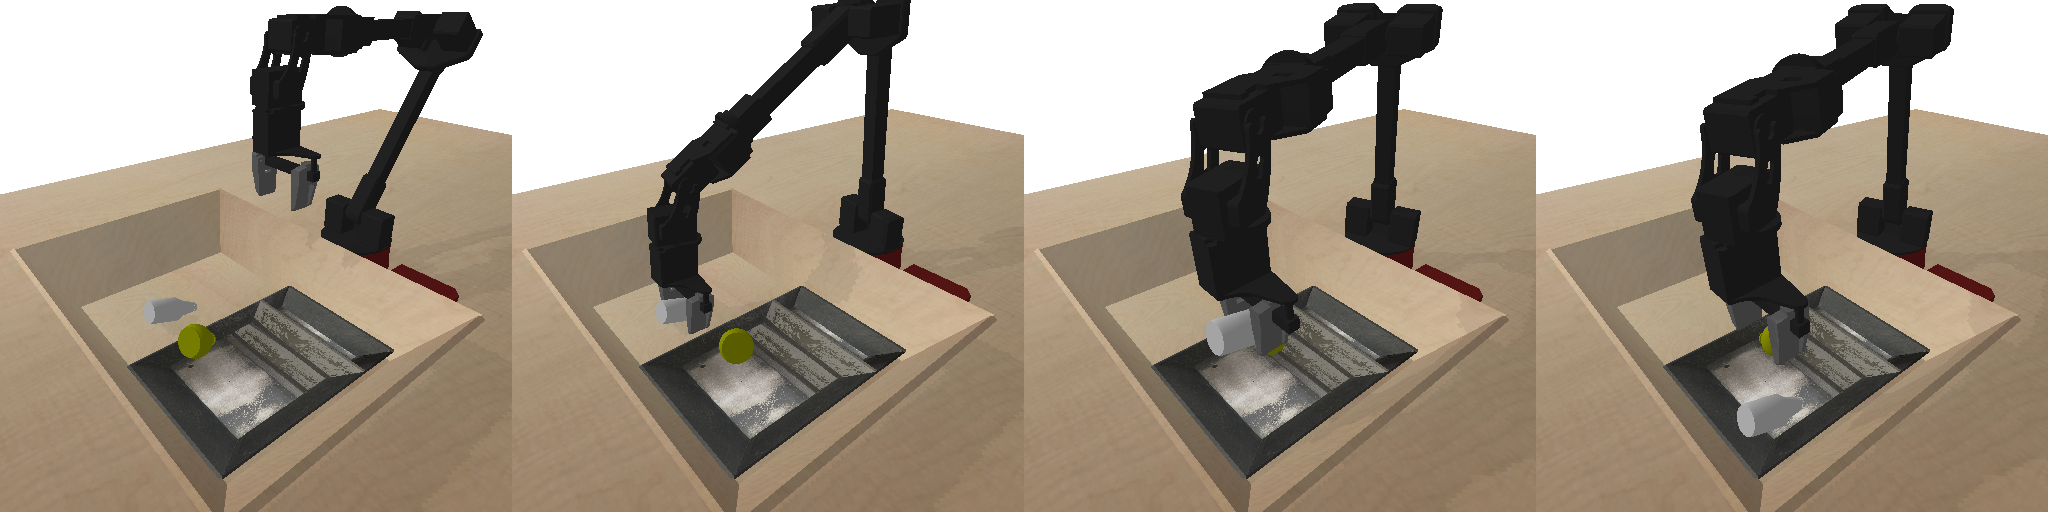}
    \caption{Example pick and place trajectory in simulation.}
    \label{fig:simulation_film}
\end{figure}

\subsection{Simulation Dataset Details}
In this section, we provide additional details on the environments and datasets used in our simulation experiments, the results for which were presented in Section~\ref{sec:simulation}. In Figure~\ref{fig:sim_objects}, we show the set of training and testing objects used in the various pick and place tasks. In Table \label{tab:env_hparams1} we provide details on number of tasks, number of episodes and other dataset properties.

\begin{figure}[!htbp]
    \centering
    \includegraphics[width=0.3\textwidth]{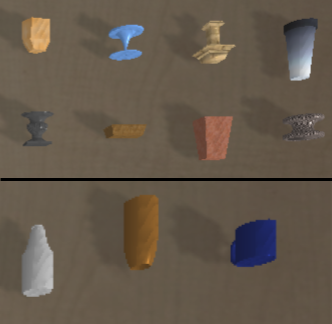}
    \caption{Simulation training (upper) and test (lower) objects. Our offline prior dataset consists of only training objects.}
    \label{fig:sim_objects}
\end{figure}

\begin{table}[!htbp]
    \begin{center}
    \begin{tabular}{lr}
    \hline
     Attribute & Value\\
    \hline
     Timesteps per Offline Trajectory & 30 \\
     Timesteps per Exploration Trajectory & 40 \\
     Forward Tasks & 8 \\
     Backward Tasks & 8 \\
     Number of Trajectories Per Task & 512 \\
    \hline
    \end{tabular}
    \end{center}
    \caption{Simulated Tasks Prior Data Details}
    \label{tab:env_hparams1}
\end{table}

\subsection{Real-World Dataset Details}

In this section, we provide additional details in Tables~\ref{tab:env_hparams2} and~\ref{tab:env_hparams3} on the environments and datasets used in our real world experiments, the results for which were presented in Section~\ref{sec:real_exps}. The real-robot dataset consists of a carefully-selected set of stuffed animals, rigid shapes, and more visually-complex toys. We utilize scripted policies in order to collected a large amount of data interacting with these objects.In the container environment, there two objects in the scene at once to provide better task specification.

\begin{table}[h]
    \begin{center}
    \begin{tabular}{lr}
    \hline
     Attribute & Value\\
    \hline
     Timesteps per Offline Trajectory & 15 \\
     Timesteps per Exploration Trajectory & 20 \\
     Forward Tasks & 20 \\
     Backward Tasks & 20 \\
     Number of Trajectories Per Task & 500 \\
    \hline
    \end{tabular}
    \end{center}
    \caption{Real-world Pick and Place Prior Data Details}
    \label{tab:env_hparams2}
\end{table}

\begin{table}[h]
    \begin{center}
    \begin{tabular}{lr}
    \hline
     Attribute & Value\\
    \hline
     Timesteps per Offline Trajectory & 30 \\
     Timesteps per Exploration Trajectory & 35 \\
     Forward Tasks & 4 \\
     Backward Tasks & 4 \\
     Number of Trajectories Per Task & 150 \\
    \hline
    \end{tabular}
    \end{center}
    \caption{Real-world Drawer Prior Data Details}
    \label{tab:env_hparams3}
\end{table}
\subsection{Generalization Test Objects}
To test the generalization performance of our fine-tuned policy, we utilize 6 different objects depicted in Figure~\ref{fig:gemeralization_objects}. The top 3 objects are used for testing the robustness of the tiger container policy, while the bottom 3 objects are for the drawer task. Note that although the objects chosen to test drawer generalization are seen in the training set for the container task, they are not contained in the offline buffer for the drawer task.

\begin{figure}[!htbp]
    \centering
    \includegraphics[width=0.4\textwidth]{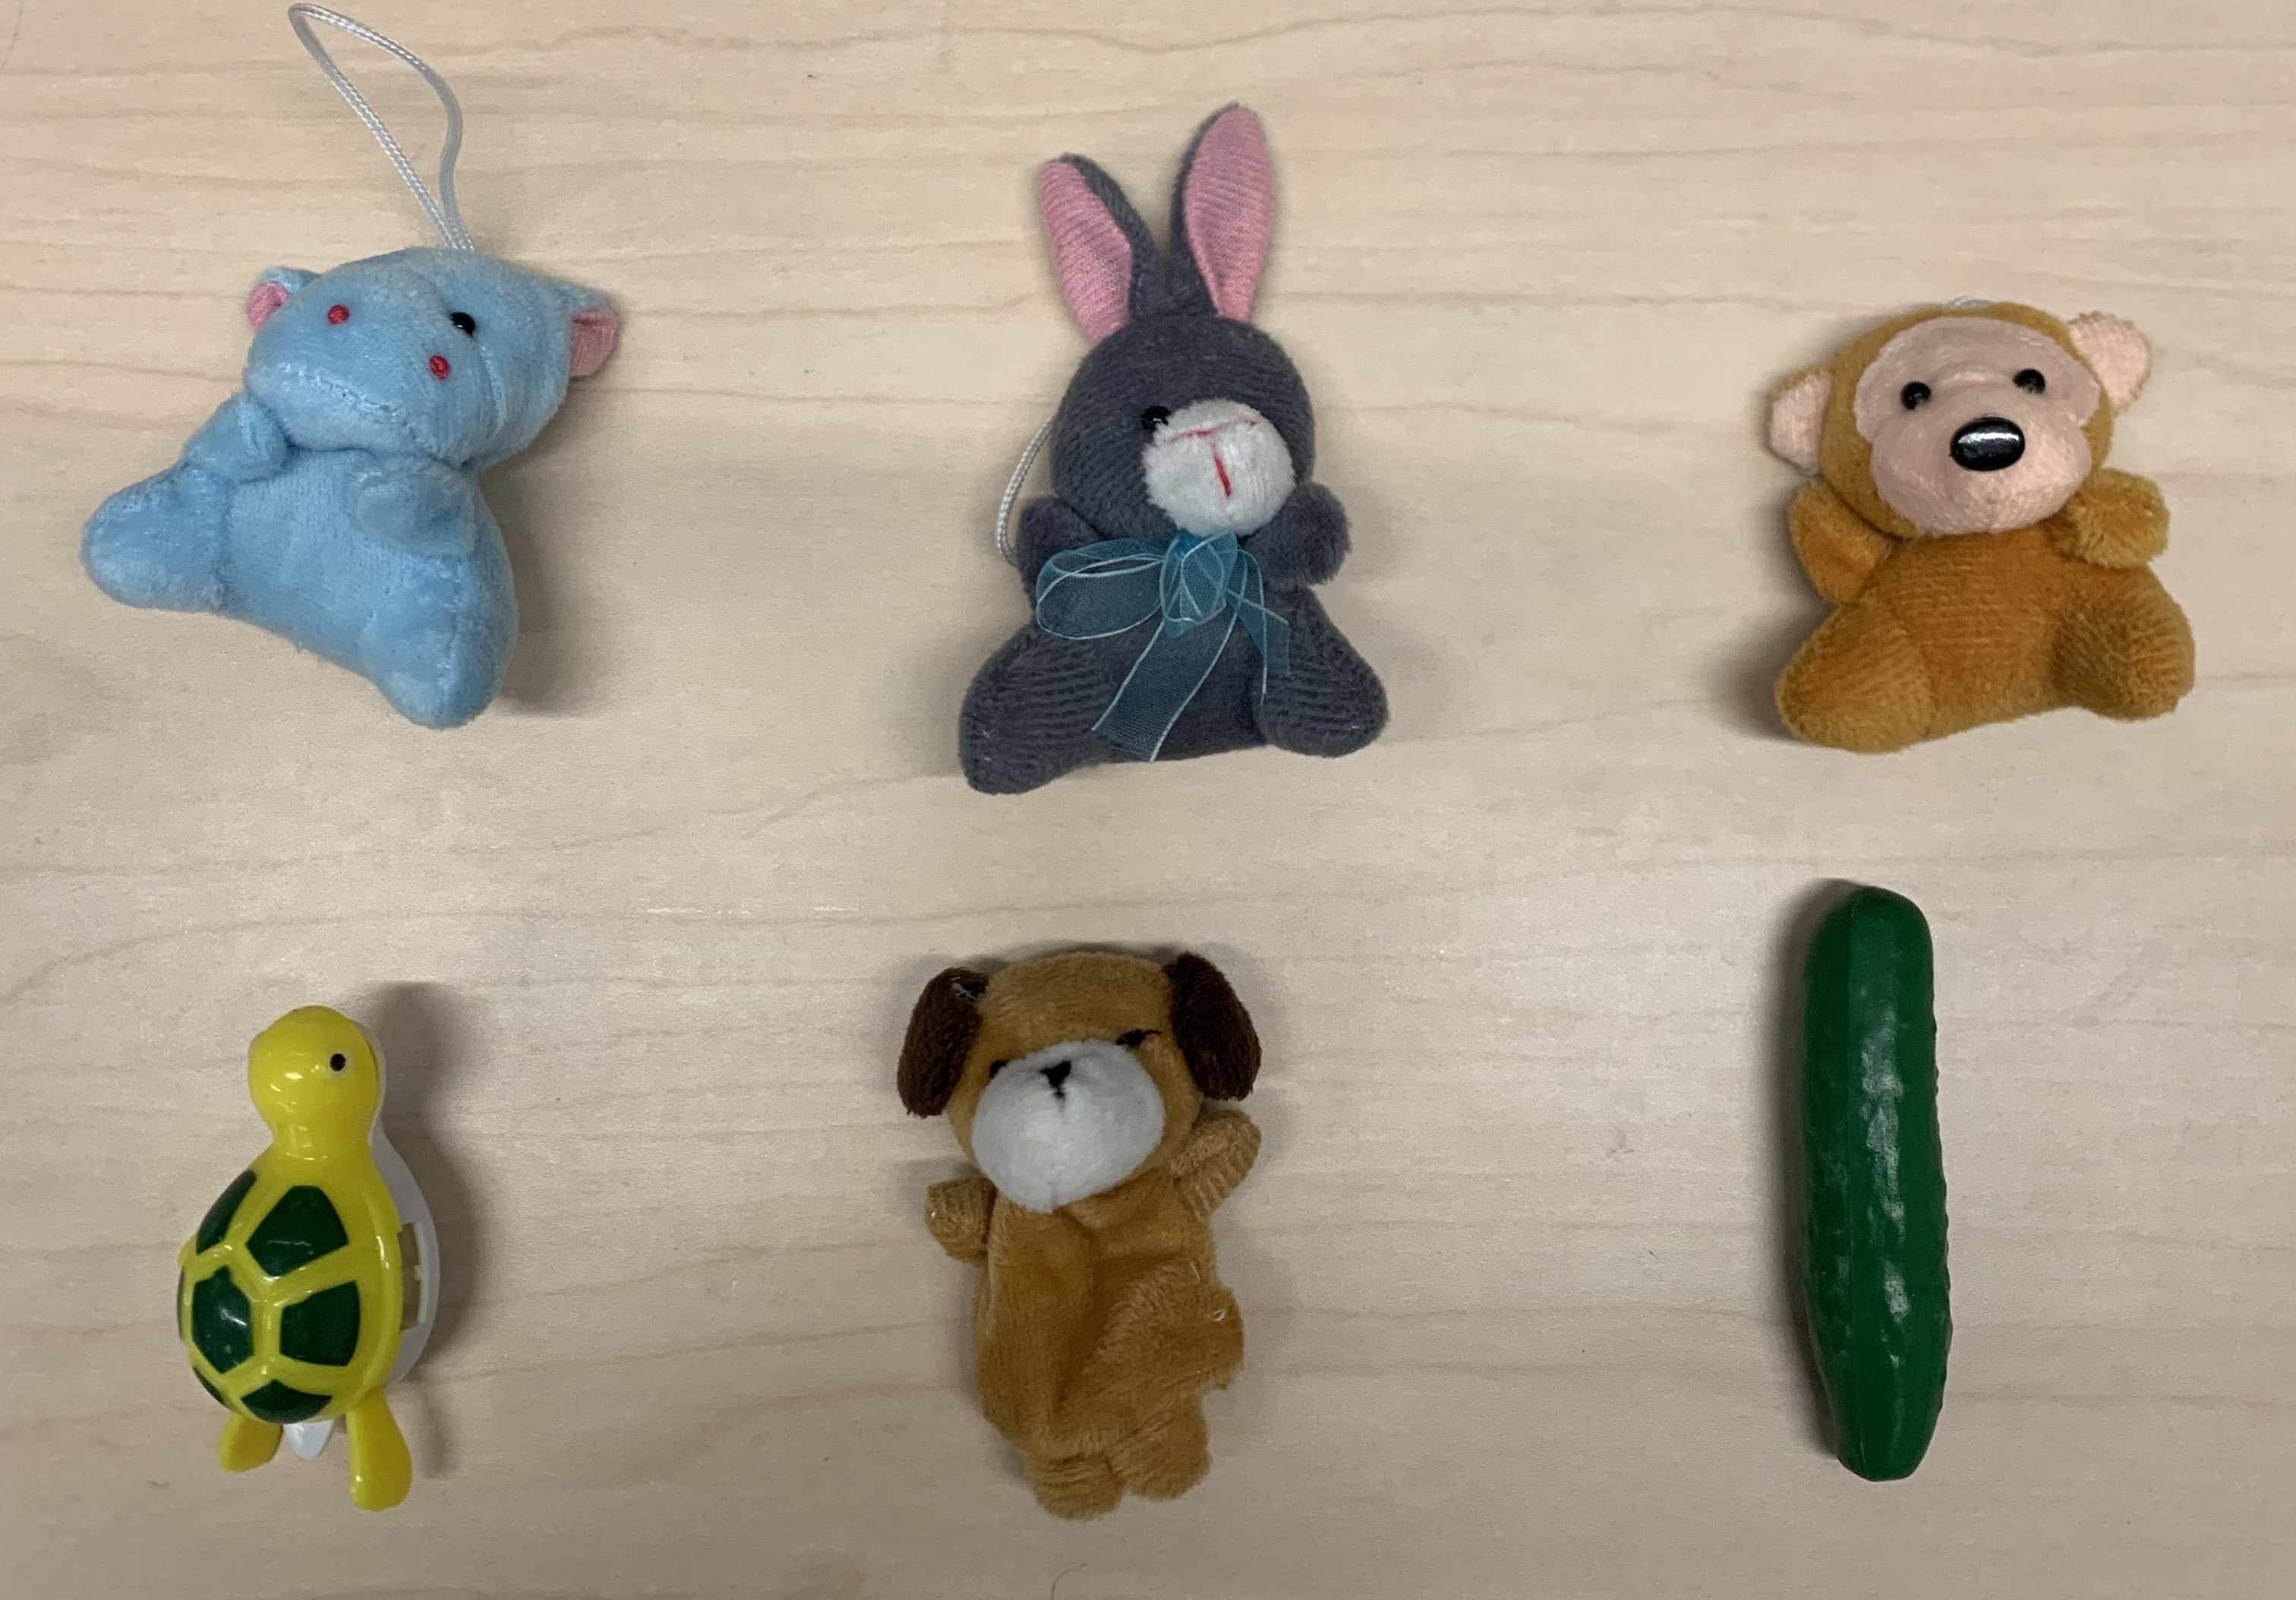}
    \caption{Generalization objects for tiger (upper) and drawer (lower) tasks.}
    \label{fig:gemeralization_objects}
\end{figure}

\subsection{Architecture Details}
In Table~\ref{tab:arch_hparams}, we provide details of the CNN architecture used for our policy and Q-function networks.
% variant['cnn_params'] = dict(
%         input_width=48,
%         input_height=48,
%         input_channels=3,
%         kernel_sizes=[3, 3, 3],
%         n_channels=[16, 16, 16],
%         strides=[1, 1, 1],
%         hidden_sizes=[1024, 512, 256],
%         paddings=[1, 1, 1],
%         pool_type='max2d',
%         pool_sizes=[2, 2, 1],  # the one at the end means no pool
%         pool_strides=[2, 2, 1],
%         pool_paddings=[0, 0, 0],
%         image_augmentation=True,
%         image_augmentation_padding=4,
%     )

\begin{table}[!htbp]
    \begin{center}
    \begin{tabular}{lr}
    \hline
     Attribute & Value\\
    \hline
     Input Width & 48 \\
     Input Height & 48 \\
     Input Channels & 3 \\
     Kernel Sizes & [3, 3, 3] \\
     Number of Channels & [16, 16, 16] \\
     Strides & [1, 1, 1] \\
     Fully Connected Layers & [1024, 512, 256] \\
     Paddings & [1, 1, 1] \\
     Pool Type & Max 2D \\
     Pool Sizes & [2, 2, 1] \\
     Pool Strides & [2, 2, 1] \\
     Pool Paddings & [0, 0, 0] \\
     Image Augmentation & Yes \\
     Image Augementation Padding & 4 \\ 
    \hline
    \end{tabular}
    \end{center}
    \caption{CNN Architecture for Policy and Q-function networks}
    \label{tab:arch_hparams}
\end{table}

% \subsection{Real-world Reset-Free Fine-tuning Success Rate Plots}
% In this section, we provide the reset-free fine-tuning success rates for real-robot tasks. These plots have lower success rates than reported in the evaluation results because it can get stuck in various positions from which it is difficult for the policy to reset. Additionally, we evaluated deterministic versions of the policy, which empirically performed better than their stochastic counterparts.
% \begin{figure}[!htbp]
%     \centering
%     \includegraphics[width=0.4\textwidth]{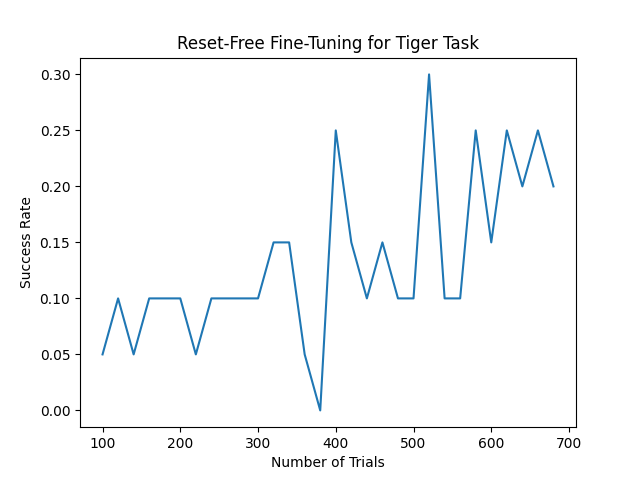}
%     \caption{Reset-free fine-tuning success rate for tiger task}
%     \label{fig:gemeralization_objects}
% \end{figure}

% \begin{figure}[!htbp]
%     \centering
%     \includegraphics[width=0.4\textwidth]{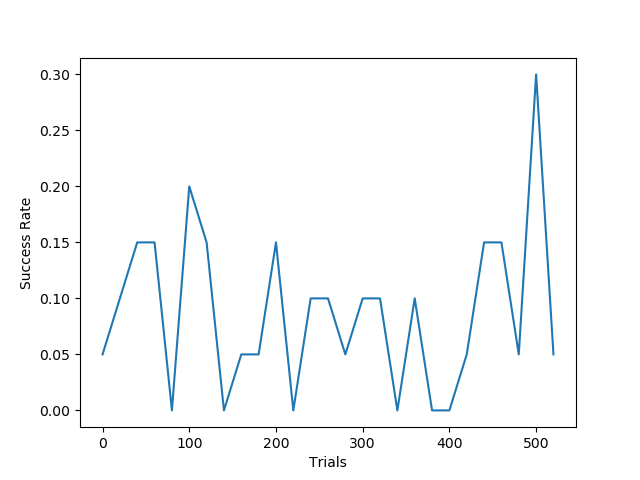}
%     \caption{Reset-free fine-tuning success rate for the task of placing a tiger object into the drawer.}
%     \label{fig:gemeralization_objects}
% \end{figure}

\subsection{Simulation Offline Success Rate Plots}
In Figure~\ref{fig:offline_rl_baselines}, we provide the learning curves for the offline phase of the \textbf{R3L} and \textbf{Multi-task RL} baselines.

\begin{figure}[!htbp]
    \centering
    \includegraphics[width=0.3\textwidth]{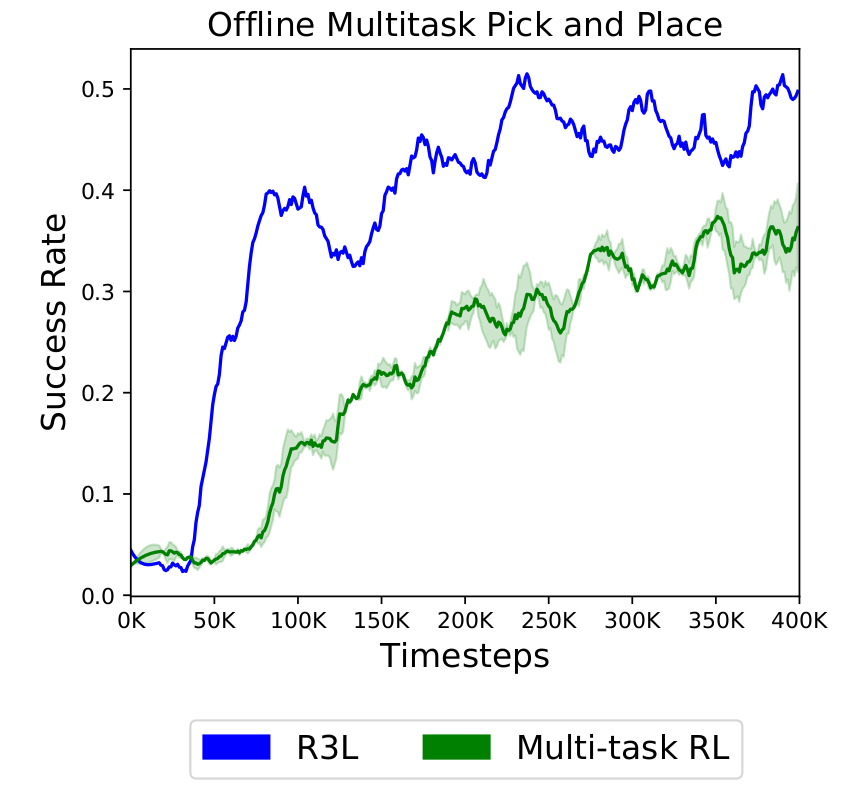}
    \caption{We see that the multitask pick and place success rates learned by our offline RL baselines show a significant amount of learning, even though they perform poorly on test tasks as seen in Figure~\ref{fig:reset_free_graphs}}.
    \label{fig:offline_rl_baselines}
\end{figure}
